# Supplementary material for: Majorana quasiparticles in semiconducting carbon nanotubes
Source: arXiv:1711.03616 ancillary file (2017-11-09)
Supplement: Supplementary file 1 [file Majorana_11-2017_supplement.pdf]

# Majorana quasiparticles in semiconducting carbon nanotubes

## Supplemental Material

Magdalena Marganska,<sup>1</sup> Lars Milz,<sup>1</sup> Wataru Izumida,<sup>1,2</sup> Christoph Strunk,<sup>3</sup> and Milena Grifoni<sup>1</sup>

<sup>1</sup>*Institute for Theoretical Physics, University of Regensburg, 93053 Regensburg, Germany*

<sup>2</sup>*Department of Physics, Tohoku University, Sendai 980 8578, Japan*

<sup>3</sup>*Institute for Experimental and Applied Physics,  
University of Regensburg, 93053 Regensburg, Germany*

- I.** Valley mixing induced by the substrate
- II.** Superconducting pairing in the four band effective model
- III.** Two band effective model
- IV.** Majorana modes at a phase boundary
- V.** Stability of the MQP against disorder
- VI.** Influence of the nearest-neighbor pairing  $\Delta_1$

### I. VALLEY MIXING INDUCED BY THE SUBSTRATE

The possibility of tunneling between the two components of a normal-superconducting (N-S) hybrid system which generates the pairing correlations in the normal part implies close contact between the N and S systems. With this close contact the N wave functions are affected by the S substrate lattice potential, registering an increased electrostatic potential in the vicinity of the N-S contact area. In order to preserve the translational symmetry of the system, which allows us to construct Bloch bands of the bulk nanotube, we treat the electrostatic potential of the substrate as a continuous ridge, adding an on-site potential term to the Hamiltonian of the CNT at the atomic sites in the proximity of the superconducting substrate. We have tested several shapes of this ridge with similar values of the resulting valley mixing energy scale,  $\Delta_{KK'}$ . For all calculations presented here we chose a Gaussian form of  $V(\varphi)$ , shown in Fig. S1a and given by

$$V(\varphi) = V_0 \exp(-(\varphi - \varphi_0)^2 / \Delta\varphi^2), \quad (\text{S1})$$

where  $\varphi$  is the angular coordinate of the nanotube atom,  $V_0$  is an arbitrarily chosen maximum height of the substrate's potential,  $\varphi_0$  is the shift between nanotube coordinates and the CNT-S contact line, and  $\Delta\varphi$  controls the sharpness of the potential. The influence of the substrate potential for three different nanotube chiralities is illustrated in Fig. S1b, where the atoms of the respective CNT's unit cell are colored according to the value of  $V(\varphi)$  at this position.

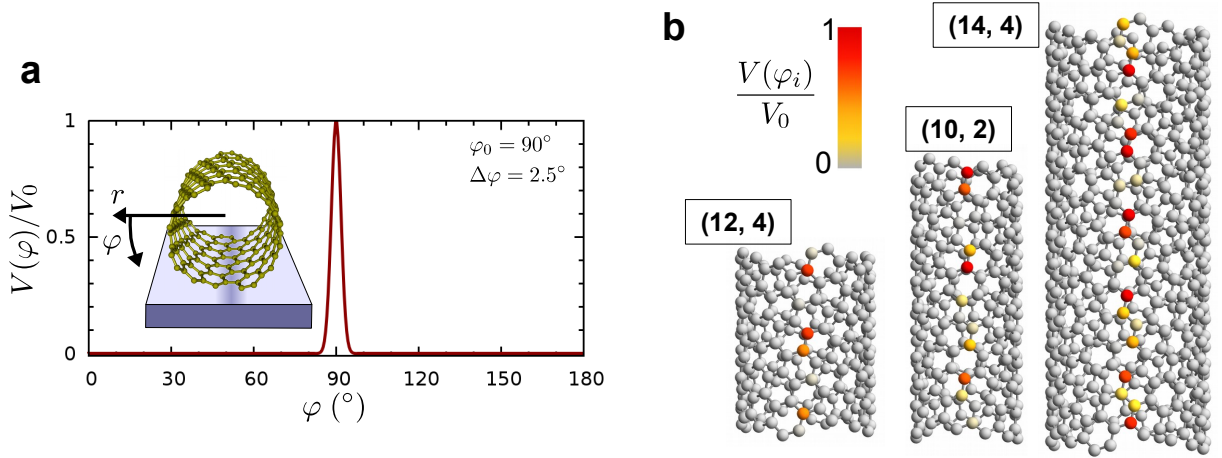

FIG. S1. **a**, The substrate potential  $V(\varphi)$  in the Gaussian form. The inset shows the nanotube coordinates in relation to the substrate. **b**, Examples of unit cells of nanotubes with different chiralities, with the atoms along the contact area colored by their value of  $V(\varphi)$ .

We shall now assess the hybridization between different momentum states in the normal CNT,  $|\mathbf{k}\rangle$  and  $|\mathbf{k}'\rangle$ . First, we introduce the basis of LCAO plane waves

$$|\mathbf{k}, p\rangle = \frac{1}{\sqrt{N_c N_L}} \sum_{\mathbf{R}} e^{i\mathbf{k} \cdot \mathbf{R}} |\mathbf{R}, p\rangle, \quad \text{with} \quad \langle \mathbf{r} | \mathbf{R}, p \rangle = p_z(\mathbf{r} - (\mathbf{R} + \delta \mathbf{R}_p)), \quad (\text{S2})$$

where  $N_L$  is the number of CNT unit cells and  $N_c$  is the number of lattice sites (graphene's unit cells) in the CNT's unit cell. The index  $p = A, B$  denotes the sublattice,  $\mathbf{R}$  are the Bravais lattice vectors and  $\delta \mathbf{R}_p$  denote the shift of the  $p$  atom from the center of graphene's unit cell. We approximate the wave functions of electronic  $p_z$  orbitals by Dirac deltas.

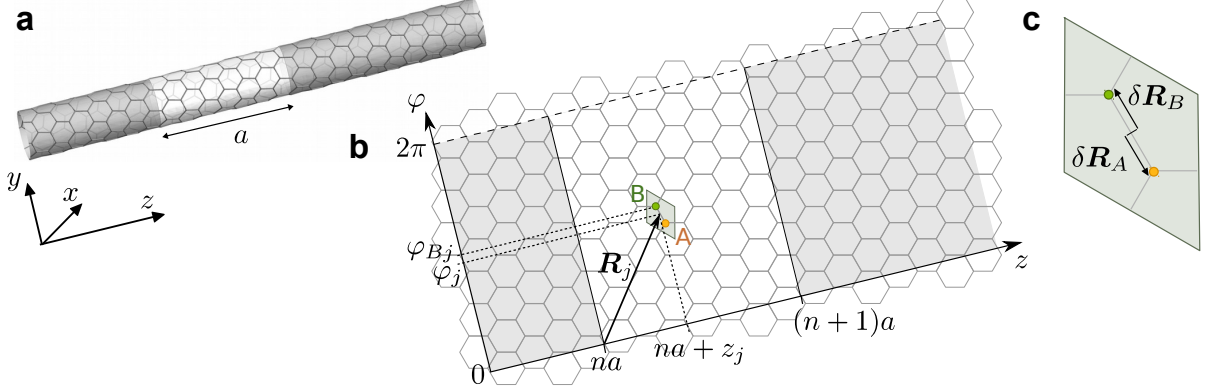

FIG. S2. **a**, Fragment of a (6,2) CNT lattice. The white area marks the translational unit cell of the CNT. **b**, Unrolled nanotube lattice and the quantities used in equations (S2) and (S3). **c**, The unit cell of graphene, with the  $A$  and  $B$  sublattice atoms and their shifts  $\delta \mathbf{R}_{A/B}$  from the center of the unit cell.

This means that our  $V(\varphi)$ , which is diagonal in position and hence diagonal in sublattice, will only yield nonzero coupling between LCAO plane waves on the same sublattice,

$$\begin{aligned} V_p(\mathbf{k}, \mathbf{k}') &:= \langle \mathbf{k}, p | V(\varphi) | \mathbf{k}', p \rangle = \frac{1}{N_c N_L} \sum_{\mathbf{R}} V(\varphi_{\mathbf{R}, p}) e^{i(\mathbf{k} - \mathbf{k}') \cdot \mathbf{R}} \\ &= \frac{1}{N_L} \sum_{n=1}^{N_L} e^{i(\mathbf{k} - \mathbf{k}') \cdot n\mathbf{a}} \frac{1}{N_c} \sum_{j=1}^{N_c} V(\varphi_{pj}) e^{i(l_{\perp} - l'_{\perp})\varphi_j} e^{i(\mathbf{k} - \mathbf{k}') \cdot \mathbf{z}_j}, \end{aligned} \quad (\text{S3})$$

where in the last step we split the sum over lattice sites  $\mathbf{R}$  into a sum over nanotube unit cells indexed by  $n$  and a sum over all atoms in one unit cell, indexed by  $j$ . The lattice constant  $a$  is the length of the CNT's unit cell,  $\varphi_j$  is the angular coordinate of the lattice site  $\mathbf{R}_j$  and  $\varphi_{pj}$  the angular coordinate of the  $p$  sublattice atom belonging to this site. The quantities  $l_{\perp}, l'_{\perp}$  are the angular momentum components of  $\mathbf{k}$  and  $\mathbf{k}'$ , respectively. The summation over the unit cells in an infinite CNT yields the selection rule for the longitudinal momentum,  $k = k'$ , while the summation over lattice sites determines the strength with which different angular momentum states at the same  $k$  are coupled. The angular momenta in the  $K$  and  $K'$  valley have opposite signs,  $l_K = -l_{K'}$ . When the  $l_K$  appropriate for a given chirality is inserted into (S3), we obtain the  $k$ -independent coupling between LCAO plane waves from  $K$  and  $K'$  valley,

$$V_{KK', p} = \frac{1}{N_c} \sum_{j=1}^{N_c} V(\varphi_{pj}) e^{2il_K \varphi_j}. \quad (\text{S4})$$

This quantity is in general complex, with different phases on the  $A$  and  $B$  sublattice, but with the same absolute value,  $|V_{KK', A}| = |V_{KK', B}| =: |V_{KK'}|$ , shown in Fig. S3. The value of  $|V_{KK'}|$  is not sensitive to the precise placement of the CNT on the substrate, i.e. to the value of  $\varphi_0$ , provided the decay angle  $\Delta\varphi$  is large enough ( $> 2 - 4^\circ$ ).

Upon conversion to the conduction/valence band basis (i.e. the basis of the CNT Bloch states) we obtain the valley mixing  $\Delta_{KK'}(k)$  which is proportional to  $|V_{KK'}|$  but depends on the value of  $k$ . As a result, the minimum of the bands is displaced from the curvature-shifted Dirac points, as can be seen by comparing the colored and grey lines in

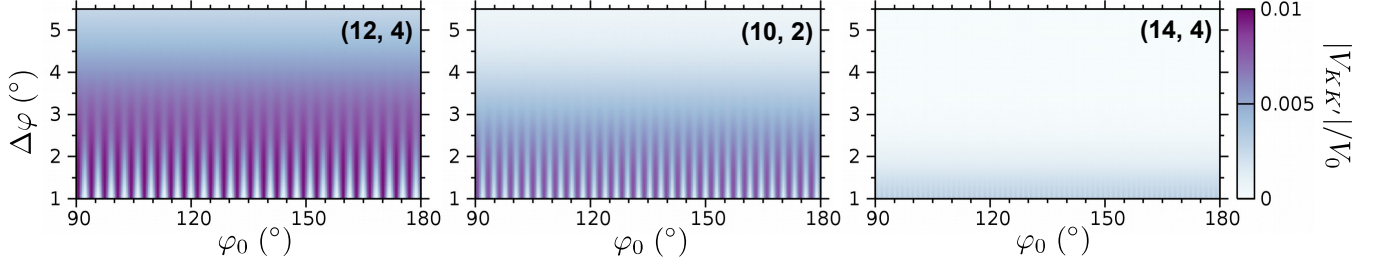

FIG. S3. Calculated plane wave coupling  $|V_{KK'}|$  as a function of the substrate potential parameters  $\varphi_0, \Delta\varphi$ . It is most effective in nanotubes with shorter unit cells, and in all of them the dependence on  $\varphi_0$  vanishes beyond some value of  $\Delta\varphi$ .

Fig. 1b in the main text. For the sake of simplicity in the effective model we accommodate this displacement through a modification of the curvature shift  $\Delta k_{\parallel}^C$ , defined in the next section, and take the value of  $\Delta_{KK'}$  to be constant in  $k$ , fitted from the width of the  $K/K'$  anticrossing in the numerically obtained band structure. This simplification eases greatly the analytical calculation, while keeping the agreement between our numerical and effective model results, as the following sections will show.

## II. SUPERCONDUCTING PAIRING IN THE FOUR BAND EFFECTIVE MODEL

When expressed in the eigenbasis of the single particle Hamiltonian (equation (15) of the Methods section), the superconducting pairing couples all four bands, though not with equal strength. The most important are the intraband pairing and interband pairing within the same pair. Reflecting the opposite spin direction  $s_z$  between  $k$  and  $-k$  states in the same band, the intraband pairing is odd in  $k$ , thus we call it  $\Delta_p$ . The interband pairing is even in  $k$  and we call it  $\Delta_s$ . The pairings with the members of the other band pair are weaker, and we call them  $\Delta'_p$  and  $\Delta'_s$ . The different pairings coupling a band ① state with positive  $k$  to the states with negative  $k$  are illustrated in Fig. S4a, and their  $k$  dependence at  $B_{\perp} = 10$  T is plotted in Fig. S4b.

The dependence of those different pairings on  $k$  and  $B_{\perp}$  is plotted in Fig. S4c. Initially with increasing field strength the spins become polarized in the  $x$  direction, thus the terms  $\Delta_p, \Delta'_s$  pairing opposite  $s_z$  spin states become on average weaker, while  $\Delta_s, \Delta'_p$  pairing opposite  $s_x$  states gain in strength. Beyond the field strength of  $\sim 20$  T the amplitude of the Zeeman term  $\mu_B B_{\perp}$  becomes comparable to that of the spin-orbit splitting and the pairing  $\Delta'_s$  mixes the two band pairs. This effect is visible in the phase diagram of Fig. 2c,e in the main text, where the upper and lower non-trivial topological region beyond  $\sim 20$  T do not overlap, but are clearly reduced. The quasiparticle energies obtained by the diagonalization of  $H + H_{SC}$  are shown in Fig. 2a of the main text.

The region which holds greatest interest for the experimental realizations is that of lower magnetic fields, in the neighborhood of  $B_c$ , i.e. the lowest field for which the energy gap closes at the  $\Gamma$  point (given by  $\mu_B B_c = 2\Delta_0 \Delta_{KK'}/\sqrt{\Delta_{SO}^2 + 4\Delta_{KK'}^2}$ ). In this regime the two band pairs can be considered independent, and we shall now construct a further simplified model which will allow us to find analytically the spectrum.

## III. TWO BAND EFFECTIVE MODEL

The four band model, while approximating very well the numerical results, is rather intractable analytically. We can simplify it, using the knowledge of the energy scales in our system. The largest relevant energy scales are  $\Delta_{SO}$  and  $\Delta_{KK'}$ , similar in magnitude, with  $\Delta_{SO} = 2$  meV and  $\Delta_{KK'} = 2.5$  meV. Two smaller energy scales are the superconducting gap  $\Delta_0 = 0.4$  meV, and the Zeeman energy  $E_Z$ . The latter can be tuned continuously, but near the boundaries of the non-trivial topological phase has similar magnitude as  $\Delta_0$ . Our strategy is therefore to diagonalize the initial single-particle Hamiltonian of the CNT (equation (10) of the Methods) together with the valley-mixing term (equation (11) of the Methods) exactly, express the Zeeman term (equation (12) in Methods) in this basis and omit the terms coupling the lower and upper band pairs. The two resulting subspaces contain only one band pair each, halving the dimensions of the Hamiltonians under our treatment.

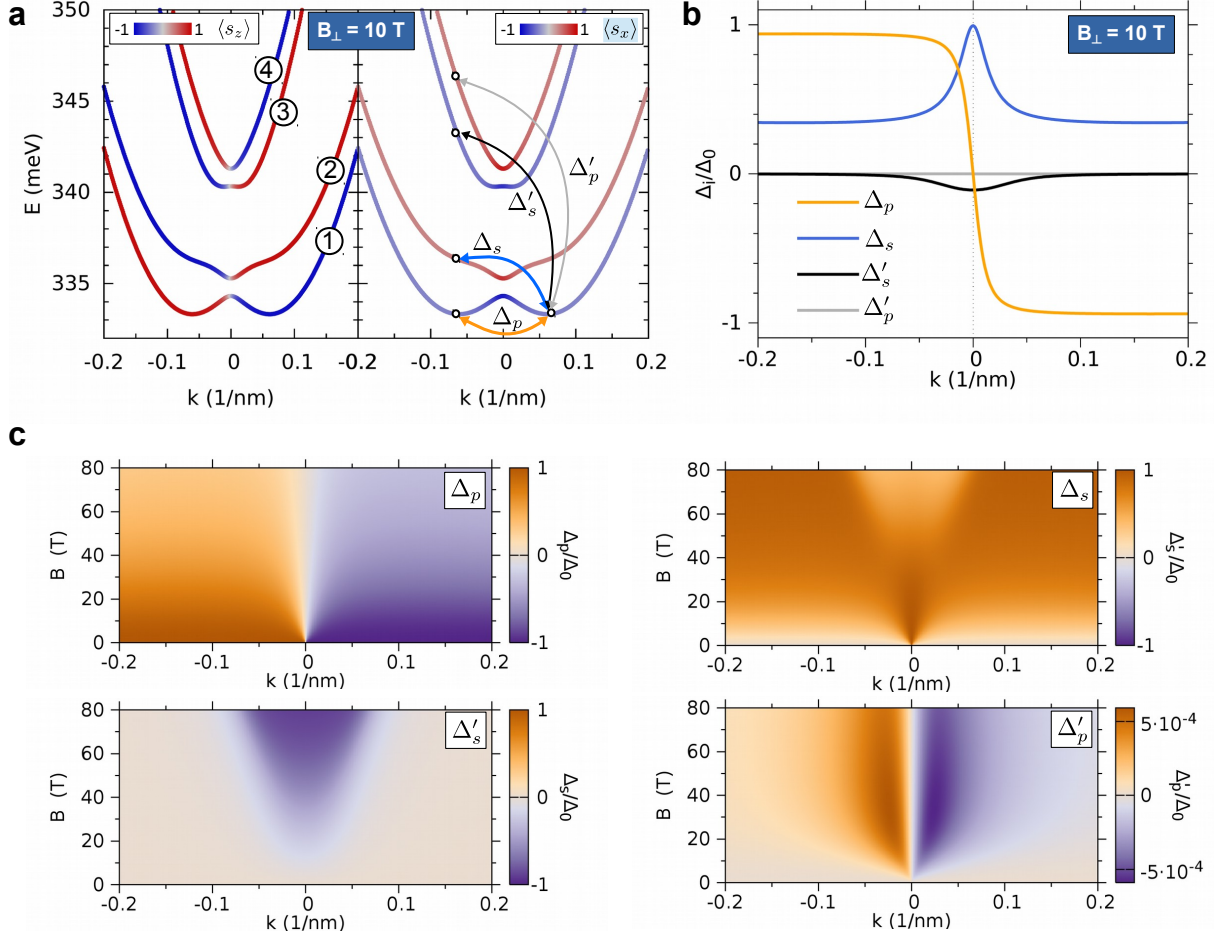

FIG. S4. **a**, The lowest four bands of a (12,4) semiconducting CNT with valley mixing and in  $B_{\perp} = 10$  T, obtained with the effective four-band model. The color scale shows the expectation value of the  $s_z$  (left panel) or  $s_x$  (right panel) component of an eigenstate's spin. The pairings between a positive  $k$  state in band ① and the four states with opposite  $k$  are indicated in the right panel. **b**, Pairing strength as a function of  $k$  for  $B_{\perp}$ , in  $\Delta_0$  units. **c**, The four pairing terms as functions of  $k$  and  $B_{\perp}$ , in  $\Delta_0$  units. Note the increase in  $\Delta'_s$  beyond  $\sim 20$  T, which couples the upper and lower band pairs.

### A. Construction of the single particle Hamiltonian

The CNT Hamiltonian  $H_{\text{CNT}} - \mu N + H_{\Delta_{KK'}}$  can be brought to a diagonal form by employing the unitary transformation

$$\begin{pmatrix} c_{kKs} \\ c_{kK's} \end{pmatrix} = \begin{pmatrix} a_s(k) & b_s(k) \\ -b_s^*(k) & a_s^*(k) \end{pmatrix} \begin{pmatrix} \alpha_{ks} \\ \beta_{ks} \end{pmatrix}, \quad (\text{S5})$$

with  $|a_s(k)|^2 + |b_s(k)|^2 = 1$ . It is diagonalized by the following values of  $a_s(k)$  and  $b_s(k)$

$$\begin{aligned} |a_s(k)|^2 &= \frac{1}{2} \left( 1 - \frac{\xi_{Ks}(k) - \xi_{K's}(k)}{\sqrt{(\xi_{Ks}(k) - \xi_{K's}(k))^2 + 4|\Delta_{KK'}|^2}} \right), \\ |b_s(k)|^2 &= \frac{1}{2} \left( 1 + \frac{\xi_{Ks}(k) - \xi_{K's}(k)}{\sqrt{(\xi_{Ks}(k) - \xi_{K's}(k))^2 + 4|\Delta_{KK'}|^2}} \right), \end{aligned} \quad (\text{S6})$$

and  $\arg(a_s(k)) = \arg(b_s(k)) = \frac{\phi}{2}$  with  $\phi = \arg(\Delta_{KK'})$ . With these we obtain

$$H_{\text{CNT}} - \mu N + H_{\Delta_{KK'}} = \sum_{k,s} E_{+s} \beta_{ks}^\dagger \beta_{ks} + E_{-s} \alpha_{ks}^\dagger \alpha_{ks}, \quad (\text{S7})$$

where the eigenvalues are defined in the following way

$$E_{\pm s}(k) = \frac{1}{2} (\xi_{Ks}(k) + \xi_{K's}(k)) \pm \frac{1}{2} \sqrt{(\xi_{Ks}(k) - \xi_{K's}(k))^2 + 4|\Delta_{KK'}|^2}. \quad (\text{S8})$$

Due to the time-reversal conjugation of  $\xi_{\tau s}(k) = \xi_{-\tau-s}(-k)$  it can be shown that  $|a_s(k)| = |b_{-s}(-k)|$  and  $E_{\pm s}(k) = E_{\pm-s}(-k)$ . These four eigenvalues are shown in Fig. S5a.

Now we will express the Zeeman term (equation (12) in Methods) in this basis:

$$H_Z = \sum_{ks} \mu_B \tilde{B}_\perp \left( \alpha_{ks}^\dagger \alpha_{k,-s} + \beta_{ks}^\dagger \beta_{k,-s} \right) + s \mu_B B_\perp^* \left( \alpha_{ks}^\dagger \beta_{k,-s} - \beta_{ks}^\dagger \alpha_{k,-s} \right).$$

where  $\tilde{B}_\perp$  and  $B_\perp^*$  are the renormalized magnetic field components. Using equations (S6) we can express them as

$$\begin{aligned} \tilde{B}_\perp &= B_\perp (|a_\uparrow(k)| |a_\downarrow(k)| + |b_\uparrow(k)| |b_\downarrow(k)|), \\ B_\perp^* &= B_\perp (|a_\uparrow(k)| |b_\downarrow(k)| - |b_\uparrow(k)| |a_\downarrow(k)|). \end{aligned} \quad (\text{S9})$$

The magnetic field  $\tilde{B}_\perp$  couples the spins within the lower and upper band pair, while  $B_\perp^*$  couples the spins between band pairs. As long as the energy difference between the lower and upper band pairs is larger than the Zeeman energy,  $\Delta E = |E_{+s} - E_{-s}| > \mu_B B_\perp$ , we can omit the terms with  $B_\perp^*$ . The upper and lower pair of bands can now be treated separately. We shall proceed to find the solutions for the lower band pair only, assuming that the chemical potential  $\mu$  is tuned into the gap between the two energy bands  $\tilde{E}_1$  and  $\tilde{E}_2$ . Therefore, we will neglect the influence of the bands  $E_3$  and  $E_4$  because those bands are not occupied. Similar calculation can be performed for the upper pair, neglecting the lower. The Hamiltonian for the two lowest energy bands is given by

$$\tilde{H}_- = \sum_{k,s} E_{-s} \alpha_{ks}^\dagger \alpha_{ks} + \mu_B \tilde{B}_\perp \alpha_{ks}^\dagger \alpha_{k,-s}. \quad (\text{S10})$$

This Hamiltonian can be diagonalized by the transformation

$$\begin{pmatrix} \alpha_{k\uparrow} \\ \alpha_{k\downarrow} \end{pmatrix} = \begin{pmatrix} s(k) & t(k) \\ -t(k) & s(k) \end{pmatrix} \begin{pmatrix} f_{k1} \\ f_{k2} \end{pmatrix}, \quad (\text{S11})$$

where the coefficients must satisfy  $s^2 + t^2 = 1$ . The new quantum number in (S11)  $i \in \{1,2\}$  just reflects the ordering of the energy bands  $E_1 < E_2$ . The coefficients  $s$  and  $t$  are defined as

$$s^2(k) = \frac{1}{2} \left( 1 - \frac{E_{-\uparrow}(k) - E_{-\downarrow}(k)}{\sqrt{(E_{-\uparrow}(k) - E_{-\downarrow}(k))^2 + 4(\mu_B \tilde{B}_\perp)^2}} \right), \quad (\text{S12})$$

$$t^2(k) = \frac{1}{2} \left( 1 + \frac{E_{-\uparrow}(k) - E_{-\downarrow}(k)}{\sqrt{(E_{-\uparrow}(k) - E_{-\downarrow}(k))^2 + 4(\mu_B \tilde{B}_\perp)^2}} \right). \quad (\text{S13})$$

The coefficients satisfy the following time-reversal conjugation  $s(k) = t(-k)$ . Then, the full Hamiltonian with decoupled band pairs in its diagonal basis is given by

$$\tilde{H}_{\text{CNT}} = \sum_k \sum_{i=1}^2 \tilde{E}_i f_{ki}^\dagger f_{ki}. \quad (\text{S14})$$

with the corresponding single-particle energies

$$\tilde{E}_i(k) = \frac{1}{2} (E_{-\uparrow}(k) + E_{-\downarrow}(k)) + (-1)^i \frac{1}{2} \sqrt{(E_{-\uparrow}(k) - E_{-\downarrow}(k))^2 + 4(\mu_B \tilde{B}_\perp)^2}. \quad (\text{S15})$$

The single-particle energies have the property  $\tilde{E}_i(k) = \tilde{E}_i(-k)$  with  $i \in \{1,2\}$  because  $\tilde{B}_\perp(k) = \tilde{B}_\perp(-k)$ . The renormalized magnetic field opens a band gap at the  $\Gamma$ -point. Fig. S5a shows the four bands  $\tilde{E}_{1/2/3/4}$  for magnetic field strengths  $B_\perp = 0, 10, 50$  T. At  $B_\perp = 10$  T the energies obtained in the two-band model still agree very well with those of the full four-band model.

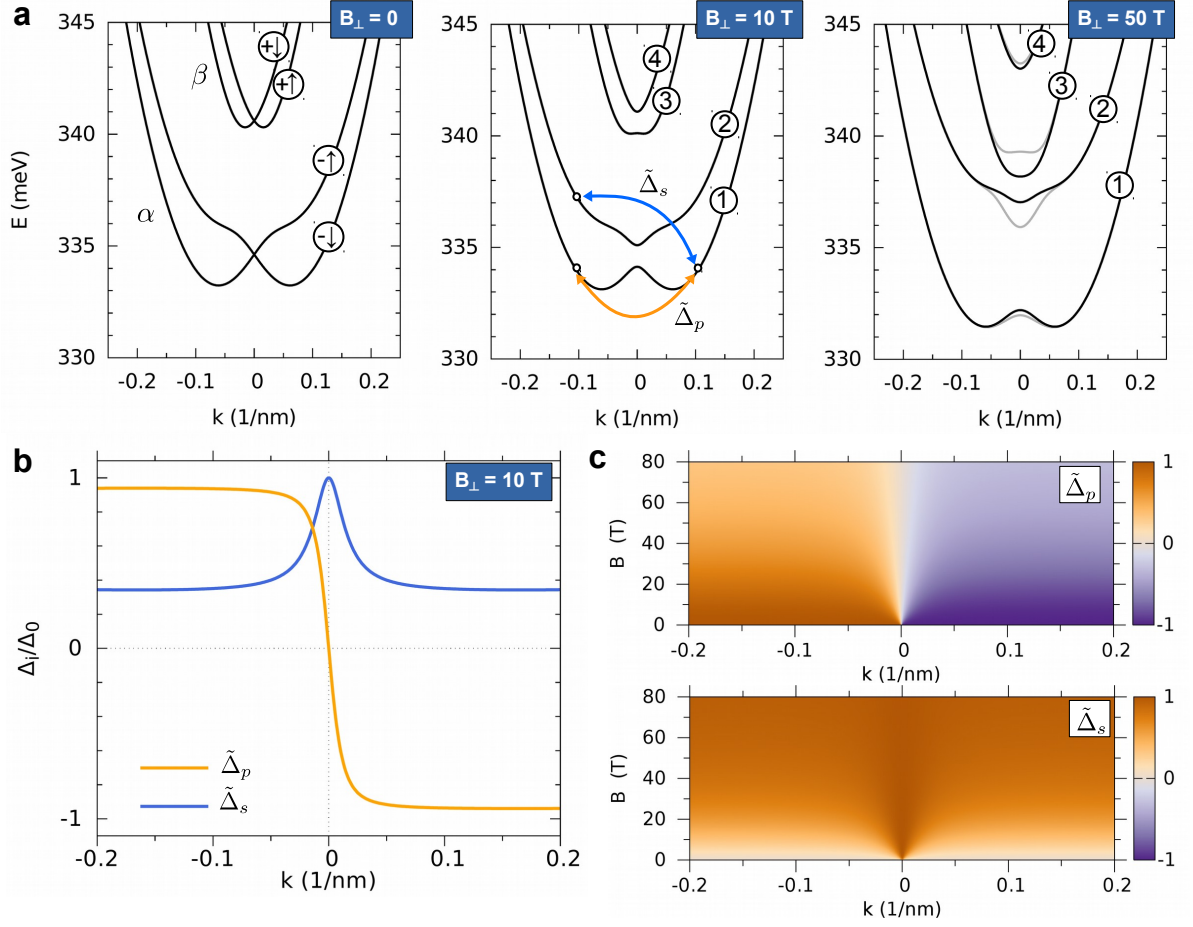

FIG. S5. **a**, The two pairs of bands  $\beta$  and  $\alpha$  with black lines showing the energies  $E_{\pm s}$ , respectively, at  $B_{\perp} = 0$ , and  $\tilde{E}_{1/2/3/4}$  at  $B_{\perp} = 10$  T and  $B_{\perp} = 50$  T. The grey lines show the corresponding solutions of the four-band model. The approximation decoupling the upper pair from the lower holds at small fields, until  $B_{\perp}^*$  becomes too large to be neglected and the two-band model becomes unreliable. Only the superconducting pairings in the same band pair are retained, with  $\tilde{\Delta}_p$  acting within band and  $\tilde{\Delta}_s$  pairing each member of the pair with its partner. **b**, The dependence on  $k$  of the two pairing terms at  $B_{\perp} = 10$  T, in  $\Delta_0$  units. **c**, The two pairing terms as functions of  $k$  and  $B_{\perp}$ . Note that the amplitude of  $\tilde{\Delta}_s$  at  $k = 0$  remains high throughout the whole  $B_{\perp}$  range, unlike in the four-band model.

## B. Superconducting pairings

Using the transformation (S5) the pairing Hamiltonian (equation (13) in the Methods section) becomes

$$H_{\text{SC}} = \sum_k \Delta_+(k) \left( \beta_{k\uparrow}^\dagger \beta_{-k\downarrow}^\dagger - \alpha_{k\uparrow}^\dagger \alpha_{-k\downarrow}^\dagger + \text{h.c.} \right) + \Delta_-(k) \left( \beta_{k\uparrow}^\dagger \alpha_{-k\downarrow}^\dagger + \alpha_{k\uparrow}^\dagger \beta_{-k\downarrow}^\dagger + \text{h.c.} \right), \quad (\text{S16})$$

where we introduce the following definition

$$\Delta_+(k) = \Delta_0 (|a_{\uparrow}(k)| |b_{\downarrow}(-k)| + |b_{\uparrow}(k)| |a_{\downarrow}(-k)|), \quad (\text{S17})$$

$$\Delta_-(k) = \Delta_0 (|a_{\uparrow}(k)| |a_{\downarrow}(-k)| - |b_{\uparrow}(k)| |b_{\downarrow}(-k)|). \quad (\text{S18})$$

For simplifications we can use the time-reversal conjugation  $|a_s(k)| = |b_{-s}(-k)|$  and by using the condition  $|a_s(k)|^2 + |b_s(k)|^2 = 1$  we obtain that  $\Delta_+(k) = \Delta_0$  and  $\Delta_-(k) = 0$ , also if  $\tilde{B}_{\perp} \neq 0$ . Only  $B_{\perp}^* \neq 0$  would induce a finite  $\Delta_-(k)$ . Since we omit  $B_{\perp}^*$ ,  $\Delta_-(k)$  is vanishing and we have again two separate pairings in the Hamiltonian. We can express the pairing Hamiltonian in the eigenbasis of the CNT with the transformation (S11) and omitting the pairing with the upper bands we obtain

$$\tilde{H}_{\text{SC}} = \sum_k \Delta_0 \left( s^2(k) f_{k1}^\dagger f_{-k1}^\dagger - t^2(k) f_{k2}^\dagger f_{-k2}^\dagger \right) + \Delta_0 s(k) t(k) \left( f_{k2}^\dagger f_{-k1}^\dagger - f_{k1}^\dagger f_{-k2}^\dagger \right) + \text{h.c.} \quad (\text{S19})$$

The Bogoliubov-de Gennes (BdG) Hamiltonian can be defined by  $\tilde{H}_{12} = \frac{1}{2} \sum_k \Psi^\dagger \tilde{\mathcal{H}}_{\text{BdG}} \Psi$  with the Nambu spinor  $\Psi^\dagger = (f_{k1}^\dagger, f_{k2}^\dagger, f_{-k1}, f_{-k2})$ . The corresponding BdG Hamiltonian for our system is given by

$$\tilde{\mathcal{H}}_{\text{BdG}} = \begin{pmatrix} \tilde{E}_1(k) & 0 & \tilde{\Delta}_p(k) & -\tilde{\Delta}_s(k) \\ 0 & \tilde{E}_2(k) & \tilde{\Delta}_s(k) & \tilde{\Delta}_p(k) \\ \tilde{\Delta}_p(k) & \tilde{\Delta}_s(k) & -\tilde{E}_1(k) & 0 \\ -\tilde{\Delta}_s(k) & \tilde{\Delta}_p(k) & 0 & -\tilde{E}_2(k) \end{pmatrix}, \quad (\text{S20})$$

with the pairing terms

$$\tilde{\Delta}_p(k) = \Delta_0 (s^2(k) - t^2(k)) = -\tilde{\Delta}_p(-k), \quad (\text{S21})$$

$$\tilde{\Delta}_s(k) = 2\Delta_0 s(k) t(k) = \tilde{\Delta}_s(-k). \quad (\text{S22})$$

We see that the pairing term  $\tilde{\Delta}_s(k)$  has an even and  $\tilde{\Delta}_p(k)$  an odd parity, as shown in Fig. S5b. We notice that these pairings depend on the magnetic field in a similar way as  $\Delta_s(k)$  and  $\Delta_p(k)$  in the four-band model, with differences visible only at high magnetic fields where the amplitude of  $\tilde{\Delta}_s(k)$  around  $k = 0$  remains large, as can be seen in Fig. S5c. From the conservation of energy it follows that  $\tilde{\Delta}_p^2(k) + \tilde{\Delta}_s^2(k) = \Delta_0^2$ .

Since  $\tilde{\Delta}_p(k=0) = 0$ , the gap closing condition can be expressed directly as

$$\tilde{\xi}_\pm(k=0) = 0, \quad (\text{S23})$$

where  $\tilde{\xi}_\pm(k) = \frac{1}{2} (\tilde{E}_1(k) - \tilde{E}_2(k)) \pm \frac{1}{2} \sqrt{(\tilde{E}_1(k) + \tilde{E}_2(k))^2 + 4\tilde{\Delta}_s^2(k)}$ . This condition, neglecting the mixing between the band pairs, is shown with dashed lines in Fig. 2c,e in the main text.

#### IV. MAJORANA STATES AT A PHASE BOUNDARY

Both the Pfaffian and the winding number invariants predict correctly whether the system is in a trivial or non-trivial topological phase, but the winding number also distinguishes between different non-trivial phases. This could be seen from Fig. 3d in the main text, where the upper and lower non-trivial regions are characterized by different values of the winding number. In consequence, if the chemical potential of the CNT is tuned in such a way that a part of the tube resides in the phase with  $\nu = -1$  and another in the  $\nu = +1$  phase, two MQP modes arise, localized at the ends of the CNT and back-to-back at the boundary between the two phases. This situation is shown in Fig. S6a,b, where the left half of the CNT is at  $\mu_L = 334.6$  meV, the right half at  $\mu_R = 340.7$  meV, the crossover region where the potential varies smoothly from  $\mu_L$  to  $\mu_R$  is of the order of 20 Å long and the magnetic field is  $B_\perp = 14$  T.

The lowest energy mode, localized at the CNT ends, is a true Majorana mode with the energy equal zero within the machine precision. Since it is composed of two parts from different topological phases, its wave function has different profile at the left and at the right end. Its left part is characterized by a single characteristic oscillation period, corresponding to the  $k_F$  of band ①, which is the single one contributing to the zero energy mode in the lower non-trivial region. The right part of the Majorana mode shows clear beating behaviour, due to the interference of contributions from ①, ② and ③ bands. The other low energy state is composed of the partners of the left and right part, located at the phase boundary. There the two modes overlap and slightly hybridize, moving the energy of the resulting state to  $\sim 1\%$  of the band gap, and skewing them from the true Majorana nature. The overlap between the two modes has however much more dramatic consequences if the two halves of the CNT are in the same phase, with an equally narrow region of trivial phase in the center, as shown in Fig. S6c,d. There the end state remains a Majorana state, but the center state hybridizes fully and moves into the bulk.

#### V. STABILITY OF THE MQP AGAINST DISORDER

Although nanotubes can now be grown with extreme cleanness [1, 2], some atoms may be adsorbed on the nanotube during the device production. We simulate their effect through a random on-site electrostatic potential, with varying concentration  $n_0 = N_{\text{imp}}/N$ , and potential strength chosen randomly from a range  $[-W_0, W_0]$ . The evolution of the quasiparticle spectra with magnetic field for two impurity concentrations and varying disorder strength is shown in Fig. S7. The nanotube and other parameters ( $\Delta_0, V(\varphi_i)$ ) are the same as in the main text.

At realistically low concentrations increasing  $V_0$  delays the onset of the zero energy mode, as can be seen from

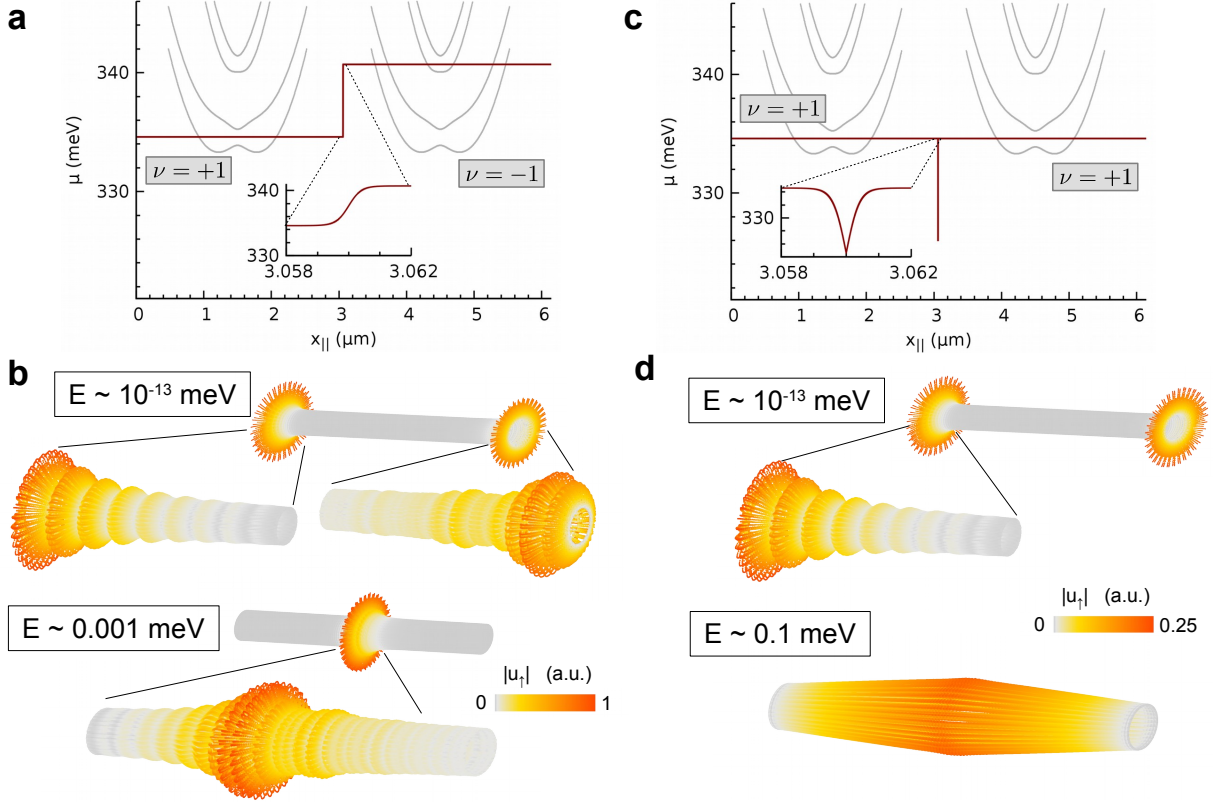

FIG. S6. **a**, The profile of the chemical potential where the left and right half of the CNT are in different non-trivial topological phases. The magnetic field is  $B_{\perp} = 14$  T and the width of the crossover region is  $\sim 20$  Å. The grey lines show for reference the energy bands. **b**, The amplitude  $|u_{\uparrow}(\mathbf{r})|$  of spin up component of the two lowest energy eigenstates. Remaining components have almost identical profiles. The state localized at the ends is a true MQP. Note different wave function profile at the left and right end, which are in different phases. The eigenstate in the center is composed of the partners of the left and right parts of the Majorana mode, which overlap and slightly hybridize, pushing the state's energy to roughly 1% of the bulk gap. **c**, The chemical potential profile for a CNT whose two halves are in the same phase, but separated by a narrow region of the trivial phase, also with the width of  $\sim 20$  Å. **d**, The amplitude  $|u_{\uparrow}(\mathbf{r})|$  of spin up component of the two lowest energy eigenstates. Remaining components have almost identical profiles. The lower energy eigenstate is a Majorana mode, the next one belongs already to the bulk, extending over the whole CNT.

(Fig. S7a,c), and perturbs the bulk bands (cf. Fig. S7c at  $W_0 = 0.6, 0.9$  eV). It also decreases the gap between the zero energy mode and the bulk states (cf. Fig S7b), but the Majorana mode is clearly present and protected, albeit it forms at higher  $B_{\perp}$  than in the clean system.

Increasing the impurity concentration beyond the realistic values, to  $n_0 = 1\%$ , as illustrated in Fig. S7d-f, is more effective at destroying the non-trivial topological phase than the increase in the disorder strength. For intermediate and large disorder strength  $W_0 \geq 0.5$  eV the formation of the zero mode occurs at much higher  $B_{\perp}$ , as can be seen from Fig. S7d,f. Even when the zero energy mode forms, it is mixed with the bulk states (cf. Fig. S7e,f), resulting in several ordinary localized states.

## VI. INFLUENCE OF THE NEAREST-NEIGHBOR PAIRING $\Delta_1$

The spin-singlet superconducting correlations can act both on-site and between nearest neighbor sites [3]. When the nearest-neighbor pairing is stronger than the on-site pairing,  $\Delta_1 > \Delta_0$ , a CNT can enter a non-trivial topological phase even in the absence of magnetic field [4], although the presence of time-reversal symmetry causes the zero energy modes to be Dirac, rather than Majorana fermions [5]. We present here the topological phase diagrams obtained with the Pfaffian technique, for the range of  $\Delta_1/\Delta_0 \leq 10$ . We keep the overall superconducting gap constant,  $\sqrt{\Delta_0^2 + \Delta_1^2} = 0.4$  meV.

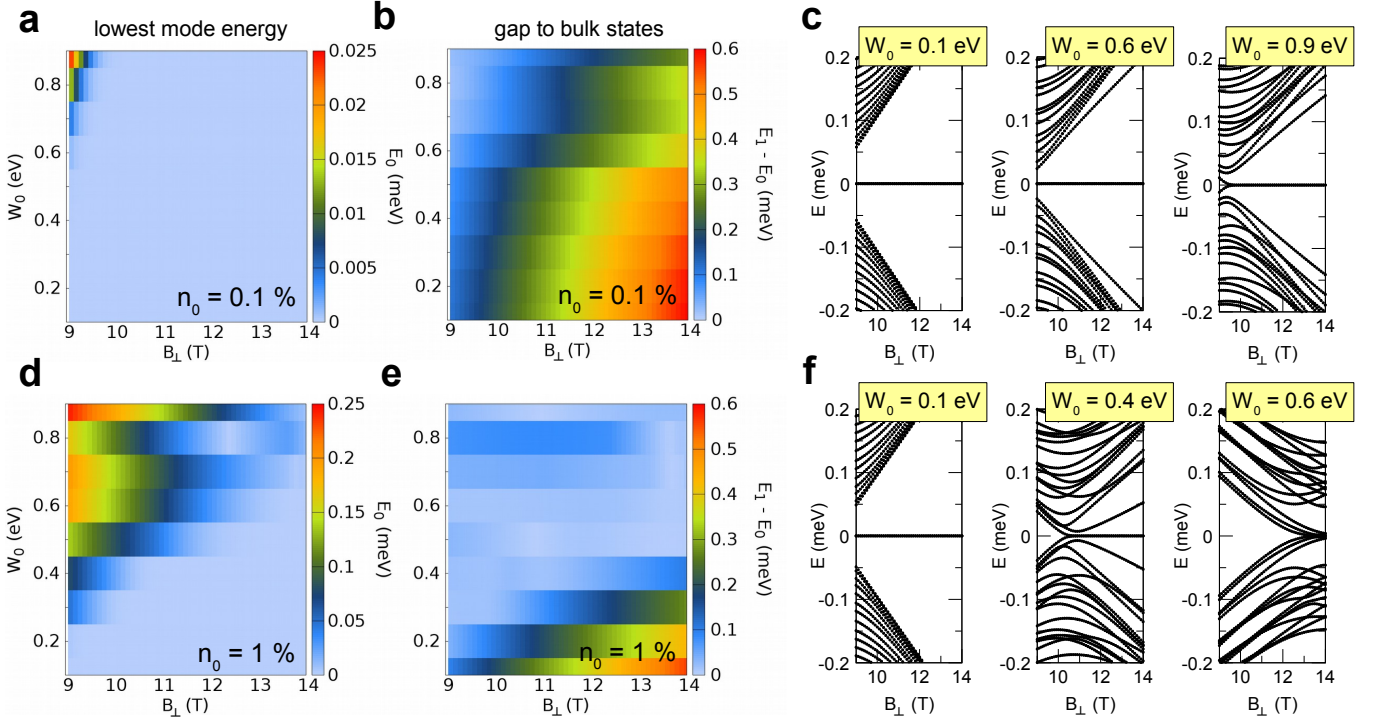

FIG. S7. **a**, The energy of the lowest positive mode  $E_0$  of the (12,4) nanotube with  $L \simeq 6 \mu\text{m}$  discussed in the main text. The chemical potential is fixed at  $\mu = 334.6 \text{ meV}$ , both the magnetic field  $B_\perp$  and the maximum disorder strength  $W_0$  vary. The latter increases in steps of  $0.1 \text{ eV}$ . In this magnetic field range the clean system is in the non-trivial topological phase. The concentration of impurities in **a-c** is  $0.1\%$ , which corresponds to 832 impurities. In all plots of this figure each value of  $W_0$  corresponds to one realization of disorder. **b**, The gap between the lowest energy mode  $E_0$  and the next,  $E_1$ . For  $E_0 \approx 0$  a large value of  $E_1 - E_0$  means wide gap between the MQP and the bulk states, indicating a stable MQP mode. **c**, Three examples of the quasiparticle spectra near  $E = 0$ . **d**, Similar to **a**, with a tenfold increase in the impurity concentration, i.e. 8320 impurities in the CNT. The concentration is the same in **d-f**. **e**, Similar to **b**. **f**, Similar to **c**.

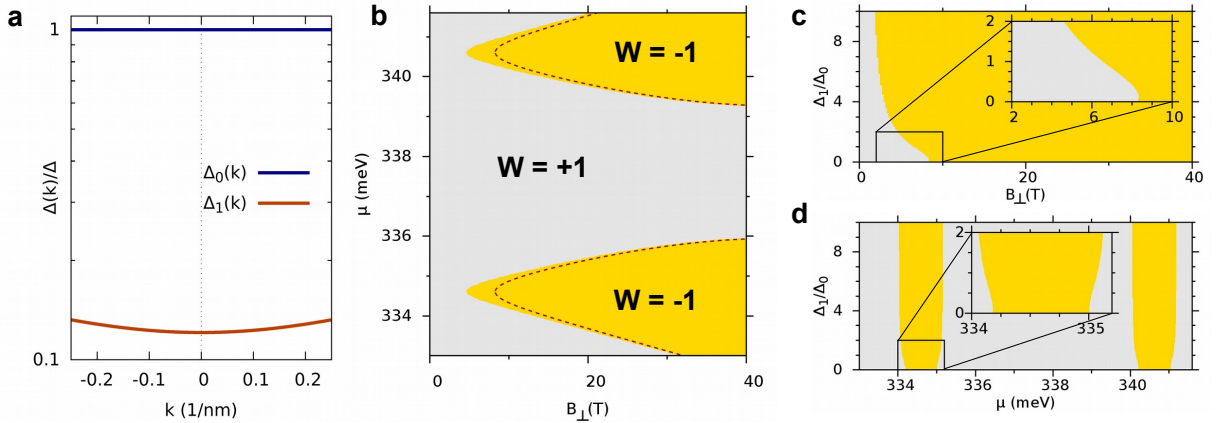

FIG. S8. **a**, The  $\Delta_0$  and  $\Delta_1(k)$  pairing strength, in the units of the appropriate pairing type, bare  $\Delta_0$  and bare  $\Delta_1$ , respectively. **b**, Topological phase diagram constructed with the Pfaffian invariant, with bare  $\Delta_1 = 2\Delta_0$ . Here and in **c,d** the value of  $\sqrt{\Delta_0^2 + \Delta_1^2}$  is kept constant and equal  $0.4 \text{ meV}$ . The red lines show the phase boundaries with  $\Delta_1 = 0$ . The inclusion of nearest neighbor pairing has extended the non-trivial region towards lower magnetic field, but otherwise its influence is invisible. **c**, Topological phase diagram at constant  $\mu = 334.6 \text{ meV}$ . Here too the increasing contribution of  $\Delta_1$  with respect to  $\Delta_0$  extends the lower border of the non-trivial phase. **d**, Topological phase diagram at  $B_\perp = 12 \text{ T}$ . Again, the inclusion of  $\Delta_1$  slightly extends the borders of the non-trivial phase.

In the basis of Bloch states the pairing  $\Delta_1$  becomes dependent on  $k$  in a way similar to  $\Delta_{KK'}$  (cf. Section I), i.e. it becomes modulated by  $|\sum_{j=1}^3 \exp(i\mathbf{k} \cdot \mathbf{\Delta R}_j)|$ , where  $\mathbf{\Delta R}_j$  are lattice vectors between unit cells to which those nearest neighbors belong. That modulation for our (12,4) CNT is plotted in Fig. S8a. The  $\Delta_0$  term remains constant in the momentum space, with its relative strength of 1 also plotted for comparison. The topological phase diagram with  $\Delta_1 = 2\Delta_0$  is shown in Fig. S8b. The non-trivial regions are extended farther towards low magnetic field, but at high  $B_\perp$  the presence of  $\Delta_1$  has no discernible influence. The topological phase diagram in the  $B_\perp, \Delta_1/\Delta_0$  plane at constant  $\mu = 334.6$  meV is shown in Fig. S8c. Again, the visible variations occur only in the low field ranges, and for low  $\Delta_1/\Delta_0$  ratios. Beyond  $\Delta_1/\Delta_0 \approx 4$  the low field boundary of the topological phase does not extend any further. Also when  $B_\perp$  is kept constant, as shown in Fig. S8d at  $B_\perp = 12$  T, the boundaries of non-trivial phase vary only slightly and mostly for  $\Delta_1/\Delta_0 < 2$ . In conclusion, the only relevant effect of  $\Delta_1$  is that it allows the MQP to form at lower magnetic field, which is a bonus for experimentalists.

- 
- [1] Jien Cao, Qian Wang, and Hongjie Dai. Electron transport in very clean, as-grown suspended carbon nanotubes. *Nat. Mater.*, 4:745, 2005.
  - [2] Lian-Mao Peng, Zhiyong Zhang, Sheng Wang, and Xuelei Liang. A doping-free approach to carbon nanotube electronics and optoelectronics. *AIP Advances*, 2(4):041403, 2012.
  - [3] Bruno Uchoa and A. H. Castro Neto. Superconducting states of pure and doped graphene. *Phys. Rev. Lett.*, 98:146801, Apr 2007.
  - [4] W. Izumida, L. Milz, M. Marganska, and M. Grifoni. Topology and zero energy edge states in carbon nanotubes with superconducting pairing. *Phys. Rev. B*, 96:125414, Sep 2017.
  - [5] Arbel Haim, Erez Berg, Karsten Flensberg, and Yuval Oreg. No-go theorem for a time-reversal invariant topological phase in noninteracting systems coupled to conventional superconductors. *Phys. Rev. B*, 94:161110, Oct 2016.
